# Supplementary material for: Privacy-Preserving Individual-Level COVID-19 Infection Prediction via Federated Graph Learning
Source: arXiv:2311.06049 source file (2023-11-10)
Supplement: Supplementary file 1 [file 7.appendix.tex]

\clearpage
\appendix
\section{Appendix}\label{sec:appendix}
\subsection{Notations of This Work}\label{par:notation}

\subsection{The Derivation Process of the Perturbation Mechanism.}\label{par:proof}
In this Section, we provide the detailed derivation process of the pertubation mechanism mentioned in Section~\ref{par:detach}.

\begin{proof}
The differential privacy can be defined as :
\begin{equation}
\operatorname{Pr}\left[\mathcal{M}\left(\mathcal{D}_i\right) \in \mathcal{S}\right] \leq e^\epsilon \operatorname{Pr}\left[\mathcal{M}\left(\mathcal{D}_i^{\prime}\right) \in \mathcal{S}\right]+\delta,
\end{equation}
and the sensitivity can be formulated as:
\begin{equation}
\Delta s_{\mathrm{U}}^{\mathcal{D}_i}=\max _{\mathcal{D}_i, \mathcal{D}_i^{\prime}}\left\|s_{\mathrm{U}}^{\mathcal{D}_i}-s_{\mathrm{U}}^{\mathcal{D}_i^{\prime}}\right\|
\end{equation}
Based on above formulation, we give the definition of $(\epsilon, \delta)$-DP, our goal is to perturb the real and pseudo location embedding. Thus the sensitive can be calculated as:
\begin{equation}
\Delta s_{\mathrm{U}}^{\mathcal{D}_i}=\max \left\|\mathcal{L}_{i, r}-\mathcal{L}_{i, f}\right\|=\max \left\|\mathcal{L}_{i, r}\right\| \leq C_l,
\end{equation}
where $\mathcal{L}_{i, r}$ and $\mathcal{L}_{i, f}$ denotes the update value of real location and fake location, respectively. As we mentioned in Section~\ref{par:detach}, $\mathcal{L}_{i, f}=0$. Thus, we deploy the clip operation for each update value of real location embedding.
Thus, the standard deviation of the Gaussian noise can be calculated as follows:
\begin{equation}
\sigma_{l}=\frac{L C_l \sqrt{2 \ln (1.25 / \delta)}}{\epsilon}
\end{equation}

\end{proof}

% \subsection{Analysis of the Computational Overhead}\label{par:obfuscation}
